# Supplementary material for: The Bond-Calculus: A Process Algebra for Complex Biological Interaction Dynamics
Source: arXiv:1804.07603 ancillary file (2018-04-30)
Supplement: Supplementary file 1 [file technical-appendix.pdf]

# The Bond Calculus: Technical appendix

Thomas Wright, Ian Stark

April 30, 2018

## Contents

**1 Syntax** **1**
1.1 Rate laws . . . 1
1.2 Sites, locations, and affinity networks . . . 2
1.3 Species and abstractions . . . 3
1.4 Mixtures . . . 4
1.5 Abstract syntax and prime species . . . 5
1.6 Bond-calculus models . . . 7

**2 Semantics** **7**
2.1 Single molecule transition semantics . . . 7
2.2 Mixture semantics . . . 9
2.3 Rate semantics for affinity networks . . . 12
2.4 Compositionality of semantics . . . 13

**3 Dynamics** **14**
3.1 Chemical reaction network extraction . . . 14
3.2 Difference matrix and vector field . . . 15
3.3 Symbolic ODE extraction . . . 17

# 1 Syntax

In this appendex we supliment the description of the bond-calculus given in the main paper, by a formal description of the language's syntax, and its mathematical semantics, whilst giving some examples of deriving the behaviour of a model.

We will start by defining the syntax of the bond calculus. First we define rate laws which specify the rates governing reactions, and then sites, locations, and affinity networks, allowing us to specify the types of reactions taking part in a system. Next we define the two levels of the calculus of agents: the species level specifying the behaviour of individual agents, and the mixture level specifying mixtures of different concentrations of each species. Finally, we define a structural congruence relation, prime species, and normal forms, allowing us to identify equivalent species and give a unique representation of a mixture.

## 1.1 Rate laws

We first define rate laws, which form the basis of our support for general kinetics. A rate law $R : \mathbb{R}^*_{\geq 0} \to \mathbb{R}$ gives the rate $R(x_1, \dots, x_n)$ of a reaction based on the concentration of each of its arguments $x_1, \dots, x_n$. We allow arbitrary mathematical functions as kinetic laws and give examples in standard mathematical notation, however, an implementation may wish to use a more specialised format (such as MathML [3]).

$$\begin{aligned} Br_2 &\longrightarrow Br + Br \\ Br + H_2 &\longrightarrow H + HBr \\ H + Br_2 &\longrightarrow Br + HBr \\ Br + Br &\longrightarrow Br_2 \end{aligned}$$

**(a)** *Linear chain of mass action reactions.*

$$H_2 \quad + \quad BR_2 \quad \longrightarrow \quad 2\,HBr$$

$$\nu = \frac{[H_2]\,[Br_2]^{1/2}}{1 + k\frac{[HBr]}{[Br_2]}}$$

**(b)** *Composite reaction and rate $\nu$.*

**Figure 1:** *Hydrogen Bromide formation process.*

**Definition 1.1** (Rate law)**.** A rate law is a function $R : \mathbb{R}^*_{\geq 0} \to \mathbb{R}$ which takes a list of positive real valued concentrations to a real valued rate.

**Definition 1.2** (Rate law family)**.** A rate law family is a function $R : \mathbb{R}^* \to \mathbb{R}^*_{\geq 0} \to \mathbb{R}$, which takes a list of rate law parameters $\mathbf{k}$ and returns a rate law $R_{\mathbf{k}} \triangleq R(\mathbf{k})$.

We already saw some common examples of kinetic laws in Section 1 of the main paper. A slightly more exotic example is given by the HBr formation process.

**Example 1.3** (Hydrogen Bromide formation)**.** Hydrogen Bromide may be formed from Hydrogen and Dibromide via the linear chain reaction shown in Figure 1a [6]. This reaction can be modelled as a single ternary reaction (shown in Figure 1b) with rate law given by,

$$L_k([H_2]\,, [Br_2]\,, [HBr]) = \frac{[H_2]\,[Br_2]^{1/2}}{1 + k\frac{[HBr]}{[Br_2]}}.$$

We will return to this example throughout this section to illustrate many features of the language and its semantics.

## 1.2 Sites, locations, and affinity networks

As the basis of a model we define the set Site of *site names*, along with the set Loc of *location names*. Sites represent (chemical) reaction sites and determine when molecules may react, whilst locations refer to internal locations within a molecule. We distinguish a special location $\top \in$ Loc, the *ambient location*, referring to the top level of a mixture. The set Name consists of located sites $\pi = s@\ell$ where $s$ is a site and $\ell$ is a location. Then two located sites $s@\ell$ and $t@m$ can interact allosterically if they are at the same location $\ell = m$, however, sites at different molecular locations may still engage in intermolecular reactions. A site $s@\top$ at the ambient location $\top$ is called an *ambient site* and we establish the shorthand $s \triangleq s@\top$; an ambient site is not involved in in allosteric interactions, but can be involved in intermolecular reactions.

In order to determine the dynamics of a system we will need to know which sites may react with which, and associate kinetic laws to these reactions. Reactions in the bond-calculus are specified by pattern matching. Clusters $\gamma = s_1 | \ldots | s_n$ match against a collection of sites in the same molecule (and specify allosteric interactions), whilst patterns $\boldsymbol{\gamma} = \gamma_1 \parallel \ldots \parallel \gamma_n$ match against solutions of molecules (in which each molecule must contain the corresponding cluster of sites). Any site can be treated as a trivial cluster, and any cluster can be treated as a trivial pattern as shown in Figure 2.

**Definition 1.4.** A *cluster* $\gamma \in$ Cluster consists of a bag $\wr s_1, \ldots, s_n \wr$ of sites $s_1, \ldots, s_n \in$ Site, and we write $\gamma = s_1 | \ldots | s_n$.

**Definition 1.5.** A *pattern* $\boldsymbol{\gamma} \in$ Pattern consists of a bag $\wr \gamma_1, \ldots, \gamma_n \wr$ of clusters $\gamma_1, \ldots, \gamma_n \in$ Cluster, and we write $\boldsymbol{\gamma} = \gamma_1 \parallel \ldots \parallel \gamma_n$. An *ordered pattern* $\boldsymbol{\gamma} = \gamma_1 \parallel \ldots \parallel \gamma_n \in$ Ordered-Pattern, is a pattern which also records the order of the site patterns, and is represented by list of clusters $(\gamma_1, \ldots, \gamma_n)$.

| Site | | Cluster | | Pattern |
|---|---|---|---|---|
| $s$ | $\subseteq$ | $\gamma = s_1 \vert \ldots \vert s_n$ | $\subseteq$ | $\boldsymbol{\gamma} = \gamma_1 \parallel \ldots \parallel \gamma_n$ |

**Figure 2:** *Sites, clusters, and patterns.*

Then the reactions which can occur in a given system are specified by an affinity network $\mathcal{A}$ which specifies a pattern for each reaction which can occur, along with its rate law.

**Definition 1.6** (Affinity network)**.** An *affinity network*,

$$\mathcal{A} = \left\{\boldsymbol{\gamma}^{(1)} \;@\; L_1, \ldots, \boldsymbol{\gamma}^{(n)} \;@\; L_n\right\} \in \textsc{Aff} \triangleq \mathcal{P}\big(\textsc{Ordered-Pattern} \times \left[\mathbb{R}^*_{\geq 0} \to \mathbb{R}\right]\big)$$

consists of a set of ordered patterns $\boldsymbol{\gamma}^{(i)} = \gamma_1^{(i)} \parallel \ldots \parallel \gamma_m^{(i)}$ together with rate laws $L_i$ (where $\mathcal{P}(X)$ denotes the powerset of $X$).

In most contexts patterns are do not have a set order so $\boldsymbol{\gamma} \parallel \boldsymbol{\delta} = \boldsymbol{\delta} \parallel \boldsymbol{\gamma}$, however, in an affinity network the order of the pattern specifies the order of the arguments of the rate law (since many non-linear rate laws are not commutative). Then each term $\boldsymbol{\gamma} = \gamma_1 \parallel \ldots \parallel \gamma_n \;@\; L$ of the affinity networks specifies a reaction involving $n$ (not necessarily distinct) species of molecules containing interactions with site clusters $\gamma_1, \ldots, \gamma_n$ at reaction rate $L([\gamma_1], \ldots, [\gamma_n])$.

**Example 1.7.** The HBr formation reaction has affinity network,

$$\mathcal{A} \triangleq \left\{h \parallel b \parallel h^*|b^* \;@\; \mathrm{L}_k\right\}$$

where the rate law $\mathrm{L}_k$ is as defined in Example 1.3.

## 1.3 Species and abstractions

We will now define the syntax rules for species in the language. In order to handle communication prefixes which bind locations such $x(\ell_1, \ldots, \ell_n).A$, we will present the calculus in an *abstraction-concretion* style following [18] (although, given the symmetry of our communication operator, we only have abstractions) and similarly to continuous $\pi$ [16], so in addition to species $A$ we define *abstractions* $F \triangleq (\ell_1, \ldots, \ell_n)S$ where the variables $\ell_1, \ldots, \ell_n$ bind locations in $S$. Then we can treat prefixes such as $x(\ell_1, \ldots, \ell_n).A$ as syntactic sugar for $x.(\ell_1, \ldots, \ell_n)A$ and thereby restrict our attention to simple communication prefixes of form $x@\ell.F$ to simplify the presentation of the language. So, we start by giving the following grammar for *species*:

$$A, B \;::=\; \mathbf{0} \;\mid\; \pi_1.F_1 + \ldots + \pi_n.F_n \;\mid\; A \,|\, B \;\mid\; (\nu\, \ell_1, \ldots, \ell_n)A \;\mid\; D(s_1, \ldots, s_n; \ell_1, \ldots, \ell_m)$$

That is, a species can be any of:

- The *null species* $\mathbf{0}$. This does exactly nothing, and represents an agent which attempts no communication actions.
- A *choice* $\pi_1.F_1 + \ldots + \pi_n.F_n$ of one of $n$ abstractions $F_1, \ldots, F_n$ guarded by the *prefixes* $\pi_1 = s_1@\ell_1, \ldots, \pi_n = s_n@\ell_n \in \mathcal{N}$. This means that the species can evolve into one of the abstractions $F_i$, but only after the synchronisation corresponding to the prefix given by the (potentially) located site $\pi_i = s_i@\ell_i$ has occurred. We define the empty choice as $\mathbf{0}$.
- A *parallel composition* $A \,|\, B$ of two species $A$ and $B$. In this species any of the evolutions of $A$ or $B$ can occur in parallel and they can communicate with each other.
- A *location binding* (or *restriction*) $(\nu\, \ell_1, \ldots, \ell_n)A$ of locations $\ell_1, \ldots, \ell_n$ in the species $A$. This marks the specified locations as local to $A$.

- A *definition application* $D(x_1, \dots, x_n; \ell_1, \dots, \ell_m)$, which applies the definition of the species $D$, supplying as arguments a list of site names $x_1, \dots, x_n$ and a list of location names $\ell_1, \dots, \ell_m$.

The case for definition applications allows us to define the species of a system as a list of mutually recursive definitions,

$$D(x_1, \dots, x_n; \ell_1, \dots, \ell_m) \triangleq P$$

where $x_1, \dots, x_n$ bind site names in $P$, and $\ell_1, \dots, \ell_m$ bind location names in $P$. We will often write $D_{\ell_1,\dots,\ell_n}$ as shorthand for $D(; \ell_1, \dots, \ell_n)$. Unlike in many presentations of the $\pi$-calculus [19] we use recursive definitions rather than a replication operator ! since this will produce much more readable biological models, and moreover unlike in the full $\pi$-calculus where the two operators are equivalent, in calculi with only internal mobility such as $\pi$I recursion can be strictly more expressive than replication [20, 24, 7].

Next, we define abstractions according to the following grammar:

$$F, G \ ::= \ (\ell_1, \dots, \ell_n)A.$$

There is only one form of abstraction, since we list all of the abstracted names at the top level, however, we will now define operators to lift parallel composition and name restriction from the process level to the abstraction level.

**Definition 1.8.** The *parallel composition* or *colocation* of abstractions $(m_1, \dots, m_p)A$ and $(m_1, \dots, m_q)B$ is defined by,

$$(\ell_1, \dots, \ell_p)A \mid (\ell_1, \dots, \ell_q)B = (\ell_1, \dots, \ell_s)(A \mid B),$$

where $s = \max\{p, q\}$. We extend this definition to all abstractions by identifying abstractions upto $\alpha$-renaming.

**Definition 1.9.** The *restriction* of names $\ell_1, \dots, \ell_p$ in an abstraction $(m_1, \dots, m_q)A$ is defined by,

$$(\nu\, \ell_1, \dots, \ell_p)(m_1, \dots, m_q)A = (m_1, \dots, m_q)(\nu\, \ell_1, \dots, \ell_p)A$$

where location names $\ell_1, \dots, \ell_p$ and $m_1, \dots, m_q$ are assumed to be distinct by $\alpha$-renaming.

We will also freely allow a species $A$ to be embedded as a trivial abstraction $()(A)$, and we can see that in this case these definitions reduce to parallel composition and restriction of species. The parallel composition operation on abstractions is similar to the *pseudo-application* operation in the abstraction-concretion presentation of the $\pi$-calculus [18, 16], but for us plays the role of combining the contributions of two parties in a reaction into a complex.

An abstraction represents the products of a open reaction, and is expanded via colocation as more reactants join the reaction. Once all the reactants have joined, an abstraction can be *committed*, giving the resulting species.

**Definition 1.10.** The *committed product* of an abstraction $F$ is the species given by,

$$\mathrm{commit}((\ell_1, \dots, \ell_n)A) \triangleq (\nu\, \ell_1, \dots, \ell_n)A.$$

## 1.4 Mixtures

Multiple species may be combined into a mixture, representing a chemical solution of different concentrations of each pure species. Mixtures are specified according to the grammar:

$$P, Q \ ::= \ c \cdot S \ \mid \ P \parallel Q$$

that is, a mixture is defined recursively as either:

- $c \cdot S$, meaning species $S$ is present in concentration $c \in \mathbb{R}_{\geq 0}$.
- The *parallel composition* or *solution* $P \parallel Q$ of two processes $P$ and $Q$.

As shorthand we may omit the dots and write $c_1 \cdot A_1 \parallel \dots \parallel c_n \cdot A_n$ as $c_1 A_1 \parallel \dots \parallel c_n A_n$.

## 1.5 Abstract syntax and prime species

In the preceding part of this section we defined a formal grammar specifying concrete syntax of the language. However, this syntax contains a lot of redundancy, allowing us to write a given species in many equivalent ways. A simple example of this is $\alpha$-equivalence: the species $(\nu\,\ell)(S^*_\ell|E^*_\ell)$ and $(\nu\,m)(S^*_m|E^*_m)$ since they differ only in the name of the bound location $\ell$, and we can express this type of equivalence as $(\nu\,\ell)(S^*_\ell \mid E^*_\ell) \equiv_\alpha (\nu\,m)(S^*_m|E^*_m)$. We need some way of identifying these equivalent processes in order to practically implement the system, since separately tracking many equivalent copies of the same species would result in a much larger (and frequently infinite) state space.

We resolve this issue by defining a *structural congruence* relation $\equiv$ on species, abstractions, and mixtures which tells us when two systems are considered syntactically equivalent. This includes $\alpha$-equivalence and a number of other equivalences specific to the language (many of these coincide with the structural congruence relations for other variants of the $\pi$-calculus [19, 16, 22]). When two species (abstractions, mixtures) are structurally congruent they are considered to be different concrete syntax, for the same abstract species (abstraction, mixture) and they may be interchanged freely.

**Definition 1.11.** The structural congruence $\equiv$ on species is the least congruence (equivalence relation, preserved all operations) containing $\alpha$-equivalence and satisfying the following axioms:

$$\begin{aligned}
\mathbf{0} \mid A &\equiv A \\
A \mid B &\equiv B \mid A \\
(A \mid B) \mid C &\equiv A \mid (B \mid C) \\
\textstyle\sum_{i=0}^{n} \pi_i.A_i &\equiv \textstyle\sum_{i=0}^{n} \pi_{\sigma_i}.A_{\sigma_i} && \text{given } \sigma \text{ perm.} \\
(\nu\,\mathbf{l} \cup \mathbf{m})F &\equiv (\nu\,\mathbf{l})(\nu\,\mathbf{m})F \\
(\nu\,\mathbf{l})F &\equiv F && \text{given } \mathbf{l} \cap \text{flocs}(F) = \varnothing \\
(\nu\,\mathbf{l})(A \mid B) &\equiv A \mid (\nu\,\mathbf{l})B && \text{given } \ell \notin \text{flocs}(F)
\end{aligned}$$

**Definition 1.12.** The structural congruence $\equiv$ on abstractions is the least congruence containing $\alpha$-equivalence and satisfying the following axioms:

$$\begin{aligned}
(\ell_1, \ldots, \ell_{n-1}, \ell_n)A &\equiv (\ell_1, \ldots, \ell_{n-1})A && \text{given } \ell_n \notin \text{flocs}(A) \\
(\ell_1, \ldots, \ell_n)A &\equiv (\ell_1, \ldots, \ell_n)B && \text{given } A \equiv B
\end{aligned}$$

**Definition 1.13.** The structural congruence $\equiv$ on processes is the least congruence containing $\alpha$-equivalence and satisfying the following axioms:

$$\begin{aligned}
(c \cdot \mathbf{0}) \parallel P &\equiv P \\
P \parallel Q &\equiv Q \parallel P \\
(P \parallel Q) \parallel R &\equiv P \parallel (Q \parallel R) \\
(c + d) \cdot A &\equiv (c \cdot A) \parallel (d \cdot A) \\
a \cdot (A \mid B) &\equiv a \cdot A \parallel a \cdot B \\
c \cdot A &\equiv c \cdot B && \text{given } A \equiv B
\end{aligned}$$

One particularly interesting case of this congruence is $a \cdot (A \mid B) \equiv a \cdot A \parallel a \cdot B$, which says that if a species (molecule) $S = A \mid B$ can be decomposed as a parallel composition of two completely independent subspecies $A$, $B$, then it in fact represents a mixture of two different species (two separate molecules). This is key to the interpretation of communication as creation and dissolution of bonds: it means two molecules will bind together as a single molecule when they gain a shared location (as in $S \parallel E \to (\nu\,\ell)(S^*_\ell|E^*_\ell)$), and a molecule will break apart when the bonds between its components are broken (as in $(\nu\,\ell)(S^*_\ell|E^*_\ell) \to S \parallel E$). In order to see how many distinct species/molecules a species actually contains, we follow continuous $\pi$ [16] (and, moreover, abstract algebra) and adopt the notion of *prime species* which cannot be broken down any further.

**Definition 1.14.** A species $S$ is *prime* if, for all species $A, B$,

$$S \equiv A \mid B \Rightarrow A \equiv \mathbf{0} \text{ or } B \equiv \mathbf{0}.$$

Any species $S$ may be decomposed as a unique parallel composition of prime species, and we denote by $\text{primes}(S)$, the bag of prime factors of $S$.

**Proposition 1.15.** *For any species $S$, we have a unique* prime decomposition*. That is, there is a unique bag of prime species* $\text{primes}(S) = \wr P_1, \ldots, P_n \wr$ *such that,*

$$S \equiv \Big|_{P \in \text{primes}(S)} P \equiv P_1 \mid \ldots \mid P_n.$$

*Proof.* This will soon follow from the normal form of Definition 1.17/Theorem 1.16 and is similar to [16, Theorem 11] (which is expanded in [15, Appendex A]). ☐

Working with structural congruence and prime species requires us to solve two several practical problems: how do we test if two species (abstractions, mixtures) are structurally congruent, and how can we concretely represent an equivalence class of species (abstractions, mixtures) up to structural congruence? We answer these problems by defining a *normal form* for species, mixtures, and abstractions which gives a unique representative element to each class of structurally congruent agents. This normal form also decomposes species into compositions of prime species, and so ensures that a mixture is represented as a mixture of prime species, each corresponding to a single type of molecule.

**Definition 1.16.** The normal form for processes, species, and abstractions are defined via the following grammar,

$$
\begin{aligned}
\textsc{Mix} &::= \|_{i=1}^{n}\, \alpha_i \cdot \textsc{Prime} & \textsc{Spec} &::= |_{i=1}^{n}\textsc{Res} \\
\textsc{Res} &::= (\nu\, \ell_1, \ldots, \ell_n)\textsc{Par} & \textsc{Par} &::= |_{i=1}^{n}\textsc{Sum} \\
\textsc{Sum} &::= \textstyle\sum_{i=0}^{n} \pi.\textsc{Abst} & \textsc{Abst} &::= (\ell_1, \ldots, \ell_n)\textsc{Spec},
\end{aligned}
$$

where we stipulate the following:

- Prime consists of elements of Spec satisfying the additional condition of primeness.
- The terms in a Proc, Spec, Par, or Sum, and the order of locations in a Res are ordered lexicographically (or according to any other canonical ordering).
- The bound locations in Res or Abst are given standardized names (we can choose canonical names using De Bruijn indices).
- A mixture Mix contains no duplicate species.
- A restriction Res contains no redundant locations, and the last location of Abst is bound in Par.
- There is no partition of locations in a restriction Res which would allow it to be split into a parallel composition of two restrictions.

**Theorem 1.17.** *(Unique normal forms) Every species (abstraction, mixture) $S$ is structurally congruent to a unique normal form* $\text{nf}(S)$ *matching to form described in Definition 1.16.*

## 1.6 Bond-calculus models

We have now defined all of the components of a bond-calculus model,

**Definition 1.18.** A bond-calculus model $(\Pi_0, \mathcal{A})$ consists of

- An initial mixture $\Pi_0 \in \textsc{Mix}$.
- An affinity network $\mathcal{A} \in \textsc{Aff}$.

Here the initial mixtures $\Pi_0$ may depend on a number of species definitions, whilst the affinity network may depend on a number of kinetic law definitions.

In the spirit of compositional modelling, we are able to build models by combining models of smaller components.

**Definition 1.19.** We define the composition of bond-calculus models $(\Pi, \mathcal{A})$ and $(\Phi, \mathcal{B})$ as the model,

$$(\Pi, \mathcal{A}) \parallel (\Phi, \mathcal{B}) \triangleq (\Pi \parallel \Phi, \mathcal{A} \cup \mathcal{B}).$$

assuming the species definitions and kinetic law definitions of both models are consistent.

# 2 Semantics

In this section we will define a formal semantics for bond-calculus models. First we will focus on the individuals in each species, giving an operational semantics for the state transitions an individual may undergo upon interaction in the form of a multi-transition system. Then we will turn our attention to continuous mixtures of species, defining the transition matrix $\mathcal{T}(\Pi)$ which captures the "concentration" of each transition $A \xrightarrow{\gamma} F$ within a mixture $\Pi$, and see how it may be derived compositionally using the interaction tensor $\odot$. Finally, we will define the reaction rate vector $\mathcal{R}_{\mathcal{A}}$ which determines the rate of each reaction given an affinity network $\mathcal{A}$.

## 2.1 Single molecule transition semantics

We start by defining a semantics for the interactions which may occur in to a single molecule of a chemical species, as a multi-transition systems, with transitions labelled by a cluster of sites, and a shared location. That is, we will represent the ability to interact on site $a$ at location $\ell$ as a unitary transition,

$$A \xrightarrow{s}_{\ell} F\ ,$$

whilst internal (allosteric) interactions will build up larger, composite interactions

$$A_1 \mid \ldots \mid A_n \xrightarrow{\gamma}_{\ell} F_1 \mid \ldots \mid F_n$$

labelled with the cluster $\gamma = s_1 | \ldots | s_n$ of all of the sites involved. Whilst operational semantics for non-deterministic programming languages are frequently specified as transition systems in order to capture the fact that the quantitative rate of a chemical reaction depends on the number of copies of a given site which are present in a molecule, we need a multi-transition system, which can include multiple instances of the same reaction (multi-transition systems are also used in other quantitative process algebra semantics [10, 16]). Additionally since our transitions correspond to open reactions, where more interactions may join at any point (either within the same species, or from other reactants in a mixture), transitions go from a species $A$ to an abstraction $F$ representing the partial products of a reaction.

The definition for our multi-transition system is as follows.

$$\frac{}{\sum_{i=0}^{n} s_i@\ell_i.F_i \xrightarrow[\ell_j]{s_j} F_j}\ \textsc{Choice}_{j,n} \qquad \frac{A \equiv_\alpha B \quad B \xrightarrow[\ell]{\gamma} F}{A \xrightarrow[\ell]{\gamma} F}\ \textsc{Alpha}$$

$$\frac{A \xrightarrow[\ell]{\gamma} F}{A \mid B \xrightarrow[\ell]{\gamma} F \mid B}\ \textsc{Par-Left} \qquad \frac{A \xrightarrow[\ell]{\gamma} F}{B \mid A \xrightarrow[\ell]{\gamma} B \mid F}\ \textsc{Par-Right}$$

$$\frac{A \xrightarrow[\ell]{\gamma} F \quad D(\mathbf{x};\mathbf{l}) \triangleq A}{D(\mathbf{y};\mathbf{m}) \xrightarrow[\ell\{\mathbf{m}/\mathbf{l}\}]{\gamma} F\{\mathbf{y}/\mathbf{x},\mathbf{m}/\mathbf{l}\}}\ \textsc{Def} \qquad \frac{A \xrightarrow[\ell]{\gamma} F \quad \ell \notin \mathbf{m}}{(\nu\,\mathbf{m})A \xrightarrow[\ell]{\gamma} (\nu\,\mathbf{m})F}\ \textsc{Res}$$

$$\frac{A \xrightarrow[\ell]{\gamma} F \quad \ell \in \mathbf{m}}{(\nu\,\mathbf{m})A \xrightarrow[\top]{\gamma} (\nu\,\mathbf{m})F}\ \textsc{Del} \qquad \frac{A \xrightarrow[\ell]{\gamma} F \quad B \xrightarrow[\ell]{\delta} G \quad \ell \neq \top}{A \mid B \xrightarrow[\ell]{\gamma|\delta} F \mid G}\ \textsc{Com}$$

**Figure 3:** *Species multi-transition system rules.*

**Definition 2.1** (Multi-transition system)**.** The *multi-transition system* for bond-calculus species consists of a multiset containing the 4-tuples (that is, *transitions*)

$$\left(A \xrightarrow[\ell]{\gamma} F\right) \triangleq (A,\gamma,\ell,F) \in \textsc{Spec} \times \textsc{Group} \times \textsc{Loc} \times \textsc{Abst},$$

which are derivable according to the rules in Figure 3 (with multiplicities corresponding to the number of derivations). We will denote the multiset of transitions $A \xrightarrow[\ell]{\gamma} F$ starting from a particular species $A$ as $\mathrm{trans}(A)$.

This is specified using a small step structural operational semantics [21] according to the transition rules in Figure 3. Initial unitary transitions are induced from choices by the Choice rule, whilst the Par-Left and Par-Right rules allow them to propagate unchanged parallel compositions. The Res rule also allows transitions to move through restrictions, provided they are not at a restricted location. The Com rule allows transitions to join together and form a larger interaction. The Del provides a way for interactions at a restricted location to move through a restriction by becoming ambient interactions at the location $\top$; this means they may engage in no more internal reactions, but can still be part of reactions with other molecules. Finally, the Dfn rule expands the transitions of named species from their definitions.

**Example 2.2.** The system with species

$$A \triangleq a.A + a.A + b.B \qquad\qquad B \triangleq a.A + a.A + a.A$$

has single species transitions,

$$\mathcal{M} = \mathrm{trans}(A) \cup \mathrm{trans}(B) = \left\{\!\!\left\{ 2 \times A \xrightarrow[\top]{a} A\ ,\ 1 \times A \xrightarrow[\top]{b} B\ ,\ 3 \times B \xrightarrow[\top]{a} A \right\}\!\!\right\},$$

which are illustrated in Figure 4. The full transition system also includes multispecies transitions $A|B \xrightarrow[\top]{b} B|B$ , $A|B \xrightarrow[\top]{a} A|A$ , $A|B \xrightarrow[\top]{a|a} A|A$ , etc.

**Figure 4:** *The multi-transition system $\mathcal{M}$, visualised as a labelled multi-graph.*

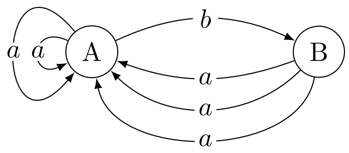


## 2.2 Mixture semantics

We will now move to the second level of the language and give a semantics for mixtures. The semantics we give is a joint extension of the vector semantics of continuous $\pi$ [16] and the numerical representation of PEPA/Bio-PEPA models [10, 12] and has also been influenced by other numerical representations [23, 13] and fluid approximation techniques [25, 5, 8]; many of the differences with existing semantics arise from the differences between the bond-calculus' communication mechanism and both binary $\pi$-calculus style communication and CSP/PEPA style multi-way cooperation. First we see how we can consider mixtures as a vector space with a basis given by prime species. Given we can decompose any species into primes, we can also decompose any mixture $\Pi$ into a unique parallel composition of prime species,

$$\Pi \equiv \alpha_1 S_1 \parallel \ldots \parallel \alpha_n S_n \equiv \sum_{S \text{ prime}} [S]_\Pi \, S$$

Then we see that mixtures form a real vector space if we define scalar multiplication of a mixture $\Pi$ by a scalar $\gamma \in \mathbb{R}$ by

$$\gamma \cdot \Pi = \gamma \sum [S]_\Pi \, S = \sum \gamma \, [S]_\Pi \, S$$

and addition of two mixtures $\Pi$ and $\Phi$ by,

$$\Pi + \Phi = \sum [S]_\Pi \, S + \sum [S]_\Phi \, S = \sum \left([S]_\Pi + [S]_\Phi\right) S = \Pi \parallel \Phi.$$

**Definition 2.3.** The mixture space $(\mathbb{M}, \cdot, +, \mathbf{0})$ is the real vector space of mixtures with scalar multiplication $\cdot$ and addition $+$ defined above.

If we define the embedding $\langle S \rangle$ of a single species as below, then we see that the vectors $\langle P \rangle$ for prime species $P$ form a basis for $\mathbb{M}$.

**Definition 2.4.** The species embedding is the map $\langle \cdot \rangle : \textsc{Spec} \to \mathbb{M}$ defined by

$$\langle S \rangle = 1 \cdot S = \sum_{P \in \text{primes } S} 1 \cdot P.$$

In order to develop our semantics we will need a number of auxilliary vector spaces for patterns, clusters, and transitions allowing us to raise the other elements of our language to the same level as the mixture space.

**Definition 2.5.** We define the following real vector spaces:

- The *pattern space* $\mathbb{P} = \textsc{Pattern} \to \mathbb{R}$ is the space of real vectors indexed by patterns.
- The *cluster space* $\mathbb{G} = \textsc{Cluster} \to \mathbb{R} \subseteq \mathbb{P}$ is the space of real vectors indexed by clusters of sites.
- The *transition space* $\mathbb{T} = \textsc{Spec} \times \textsc{Abst} \to \mathbb{R}$ is the space of real vectors indexed by transitions $A \to F \triangleq (A, F)$.

These are given the bases of indicator functions $\mathbf{I}(\gamma_1\| \dots \|\gamma_n)\,, \mathbf{I}(\gamma)\,, \mathbf{I}(A)\,, \mathbf{I}(A \to F)$ respectively, where, the indicator functions $\mathbf{I}(X) : \mathbb{X} \to \mathbb{R}$ are defined by,

$$\mathbf{I}(X)\, Y \triangleq \begin{cases} 1 & \text{if } X = Y \\ 0 & \text{otherwise} \end{cases}$$

The semantics for the language will be defined in terms of linear maps $M \in \mathcal{L}(\mathbb{P}, \mathbb{T})$ (i.e. matricies) which map pattern vectors into transition vectors. These maps correspond to a system of pattern labelled transitions representing the partial reactions arising from a given mixture, with coefficients representing the concentration of the transition. We have a basis for $\mathcal{L}(\mathbb{P}, \mathbb{T})$ consisting of the matricies $\mathbf{E}(A \to F,\, \gamma)$ defined such that

$$\mathbf{E}(A \to F,\, \gamma)\, \mathbf{I}(\gamma) \triangleq \begin{cases} \mathbf{I}(A \to F) & \text{if } \gamma = \delta \\ \mathbf{0} & \text{otherwise} \end{cases}$$

for any prime species $A$ and pattern $\gamma$.

**Example 2.6.** A simple example of a matrix encoding of transition systems is given by multi-transition systems. For example, the multi-transition system $\mathcal{M}$ from Example 2.2 may be represented as the matrix,

$$M = 2\mathbf{E}(A \to A,\, a) + \mathbf{E}(A \to B,\, b) + 3\mathbf{E}(B \to A,\, a)\,.$$

If we fix the finite bases, $\mathcal{B} = (A \to A,\, A \to B,\, B \to A)$ and $\mathcal{C} = (a, b)$ for the site space and transition space respectively, then a linear combination of patterns $\phi = m\mathbf{I}(a) + n\mathbf{I}(b)$ and a linear combination of transitions $\psi = p\mathbf{I}(A \to A) + q\mathbf{I}(A \to B) + r\mathbf{I}(B \to A)$ could be written as column vectors, whilst $M$ could be written as a matrix:

$$\phi = \begin{bmatrix} m \\ n \end{bmatrix} \qquad \psi = \begin{bmatrix} p \\ q \\ r \end{bmatrix} \qquad M = 2\begin{bmatrix} 1 \\ 0 \\ 0 \end{bmatrix}\begin{bmatrix} 1 & 0 \end{bmatrix} + \begin{bmatrix} 0 \\ 1 \\ 0 \end{bmatrix}\begin{bmatrix} 0 & 1 \end{bmatrix} + \begin{bmatrix} 0 \\ 0 \\ 1 \end{bmatrix}\begin{bmatrix} 1 & 0 \end{bmatrix} = \begin{bmatrix} 2 & 0 \\ 0 & 1 \\ 3 & 0 \end{bmatrix}.$$

Then we can find the total transition after a reaction matching the pattern $\phi = m \cdot a \parallel n \cdot b$ as,

$$M\phi = \begin{bmatrix} 2 & 0 \\ 0 & 1 \\ 3 & 0 \end{bmatrix}\begin{bmatrix} m \\ n \end{bmatrix} = m\begin{bmatrix} 2 \\ 0 \\ 3 \end{bmatrix} + n\begin{bmatrix} 0 \\ 1 \\ 0 \end{bmatrix} = m(2\mathbf{I}(A \to A) + 3\mathbf{I}(B \to A)) + n\mathbf{I}(A \to B)\,.$$

To extend this matrix encoding to quantitative transitions between mixtures we will use real valued concentrations as coefficients, rather than multiplicities.

We will now give a compositional semantics for mixtures in terms of the transition matrix $\mathcal{T}_{\mathcal{S}}(\Pi)$.

**Definition 2.7.** The *transition matrix* $\mathcal{T}(\Pi) \in \mathcal{L}(\mathbb{P}, \mathbb{T})$ is defined for any mixture $\Pi$ by

$$\mathcal{T}(\alpha A) \triangleq \alpha \sum \Big\{ \mathbf{E}(S \to F,\, \gamma) : S \in \text{primes}(A),\, S \xrightarrow[\top]{\gamma} F \Big\}$$
$$\mathcal{T}(\Pi \parallel \Phi) \triangleq \mathcal{T}(\Pi) + \mathcal{T}(\Phi)$$

First we note that $\mathcal{T} : \mathbb{M} \to \mathcal{L}(\mathbb{P}, \mathbb{T})$ is a linear map, with entries representing the concentration of the transitions at a given cluster. The transition matrix only contains the transitions which are possible from a prime species and which are labelled by clusters, whilst it omits composite transitions from general species which are labelled by general patterns. However, we will build up all of the possible $n$-way interactions between the species of $\Pi$ step by step using the bilinear map $\odot$ defined as follows.

**Definition 2.8.** The *interaction tensor* is the bilinear map $\odot : \mathcal{L}(\mathbb{P}, \mathbb{T}) \times \mathcal{L}(\mathbb{P}, \mathbb{T}) \to \mathcal{L}(\mathbb{P}, \mathbb{T})$ defined by,

$$\mathbf{E}(A \to F,\, \boldsymbol{\gamma}) \odot \mathbf{E}(B \to G,\, \boldsymbol{\delta}) \triangleq \mathbf{E}(A|B \to F|G,\, \boldsymbol{\gamma}\|\boldsymbol{\delta})$$

Then the interaction tensor composes transitions (representing open multi-way interactions) $A \xrightarrow{\boldsymbol{\gamma}} F$ and $B \xrightarrow{\boldsymbol{\delta}} G$ into larger open multi-way interactions, $A|B \xrightarrow{\boldsymbol{\gamma}\|\boldsymbol{\delta}} F|G$ which can be composed again as more agents join. The bilinearity of this map means that the concentration of composite transition is assumed to be the product of the concentrations of the reactants – in the mass action case this is proportional to the reaction rate, and even under general kinetic laws, this measures the availability of the reactants (in the space of possible combinations of reactants), although this may no longer correspond directly to the reaction rate. We note that finite dimensional matrices form a commutative algebra under $\odot$ with identity $\mathbf{1} = \mathbf{E}(\mathbf{0} \to \mathbf{0}, \varnothing)$, which can be completed to form an algebra of infinite dimensional matrices.

Now we see that the full transition system, containing all possible $n$-way interactions between species in $\Pi$ can be generated using the exponential function (with respect to $\odot$) as follows

$$\exp_{\odot}(\mathcal{T}(\Pi)) \triangleq \sum_{n=0}^{\infty} \frac{1}{n!}\mathcal{T}(\Pi)^{\odot n} = \mathbf{1} + \mathcal{T}(\Pi) + \frac{1}{2}\mathcal{T}(\Pi) \odot \mathcal{T}(\Pi) + \frac{1}{6}\mathcal{T}(\Pi) \odot \mathcal{T}(\Pi) \odot \mathcal{T}(\Pi) + \dots$$

That is, the transition matrix $\mathcal{T}(\Pi)$ exponentially generates the transitions of $\Pi$ (under product $\odot$).

We now see that the transition matrix gives us a practical way of finding the reactions of a system, since $\exp_{\odot}(\mathcal{T}(\Pi))\mathbf{I}(\boldsymbol{\gamma}) = \sum_{n=0}^{\infty} \frac{1}{n!}\mathcal{T}(\Pi)^{\odot n}\mathbf{I}(\boldsymbol{\gamma}) = \sum_j \alpha_j \mathbf{I}(A_j \to F_j)$ gives the vector of concentrations of all transitions matching pattern $\boldsymbol{\gamma}$ and moreover, this sum is finite since $\mathcal{T}(\Pi)^{\odot n}\mathbf{I}(\boldsymbol{\gamma})$ is zero for $n > |\boldsymbol{\gamma}|$. Furthermore, the following result assures us composition of transition matrices is equivalent to composition of transition systems.

**Proposition 2.9.** *For any mixtures* $\Pi$ *and* $\Phi$ *we have that*

$$\exp_{\odot}(\mathcal{T}(\Pi \parallel \Phi)) = \exp_{\odot}(\mathcal{T}(\Pi)) \odot \exp_{\odot}(\mathcal{T}(\Phi)).$$

*Proof.* This follows by the linearity of $\mathcal{T}$ and the fact that $\exp_{\odot}$ is multiplicative. □

*Remark* 2.10. An efficient implementation of the semantics should only compute the coefficients of the terms of $\exp_{\odot}(\mathcal{T}(\Pi))$ which actually correspond to patterns in the affinity network $\mathcal{A}$. This can be achieved either by computing $\exp_{\odot}(\mathcal{T}(\Pi))$ lazily, or by setting $\mathbf{E}(A \to F, \boldsymbol{\gamma}) = \mathbf{0}$ unless $\boldsymbol{\gamma} \subseteq \boldsymbol{\delta}$ for some $\boldsymbol{\delta} \mathbin{@} f \in \mathcal{A}$.

**Example 2.11.** Suppose we have a single species $A$ which can engage in reactions with itself,

$$A \triangleq a.A + b.B.$$

according to the affinity network,

$$\mathcal{A} = \{a \parallel b \mathbin{@} L,\, b \parallel b \mathbin{@} M\}.$$

This system has transition matrix,

$$\mathcal{T}([A]\,A) = [A]\,\mathbf{E}(A \to A,\, a) + [A]\,\mathbf{E}(A \to A,\, a)$$

From which we see which we see,

$$\begin{aligned}
\exp_{\odot}(\mathcal{T}([A]\,A))\mathbf{I}(a \parallel b) &= \mathbf{1}\mathbf{I}(a \parallel b) + \mathcal{T}([A]\,A)\mathbf{I}(a \parallel b) + \frac{1}{2}(\mathcal{T}([A]\,A) \odot \mathcal{T}([A]\,A))\mathbf{I}(a \parallel b) \\
&\quad + \underbrace{\frac{1}{6}(\mathcal{T}([A]\,A) \odot \mathcal{T}([A]\,A) \odot \mathcal{T}([A]\,A))\mathbf{I}(a \parallel b) + \dots}_{=\mathbf{0}} \\
&= \frac{1}{2}\,[A]^2\,(\mathbf{E}(A|A \to A|B,\, a \parallel b) + \mathbf{E}(A|A \to B|A,\, b \parallel a))\mathbf{I}(a \parallel b) \\
&= [A]^2\,\mathbf{I}(A|A \to A|B)\,.
\end{aligned}$$

whilst

$$\begin{aligned}\exp_{\odot}(\mathcal{T}([A]\,A))\mathbf{I}(a \parallel a) &= \frac{1}{2}\,[A]^2\,\mathbf{E}(A|A \to A|A,\, a \parallel a)\,\mathbf{I}(a \parallel b)) \\ &= \frac{1}{2}\,[A]^2\,\mathbf{I}(A|A \to A|B)\,.\end{aligned}$$

This shows that the concentration of the homogeneous self-interaction of the site $a$ with itself is halved, whilst the concentration of interaction between sites $a$ and $b$ is not, consistiently with the combinatorics of the law of mass action.

**Example 2.12.** In the HBr formation process we have species,

$$\mathrm{H}_2 \triangleq h(\ell, m).\Big(\mathrm{H}^{(\ell)} \mid \mathrm{H}^{(m)}\Big) \qquad \mathrm{H}^{(\ell)} \triangleq h^{*}@\ell.\mathrm{H}^{(\ell)}$$

$$\mathrm{Br}_2 \triangleq b(\ell, m).\Big(\mathrm{Br}^{(\ell)} \mid \mathrm{Br}^{(m)}\Big) \qquad \mathrm{Br}^{(\ell)} \triangleq b^{*}@\ell.\mathrm{Br}^{(\ell)}$$

and the dynamic complex,

$$\mathrm{HBr} = (\nu\,\ell)\Big(\mathrm{H}^{(\ell)} \mid \mathrm{B}^{(\ell)}\Big)\,.$$

Then a general mixture may be written as

$$\Pi \triangleq [\mathrm{H}_2]\,\mathrm{H}_2 \parallel [\mathrm{Br}_2]\,\mathrm{Br}_2 \parallel [\mathrm{HBr}]\,\mathrm{HBr}$$

We see that interaction matrix of the system is

$$\begin{aligned}\mathcal{T}(\Pi) = [\mathrm{H}_2]\,\mathbf{E}\Big(\mathrm{H}_2 \to (\ell, m)\Big(\mathrm{H}^{(\ell)}|\mathrm{H}^{(m)}\Big),\, h\Big) + [\mathrm{Br}_2]\,\mathbf{E}\Big(\mathrm{Br}_2 \to (\ell, m)\Big(\mathrm{Br}^{(\ell)}|\mathrm{Br}^{(m)}\Big),\, b\Big) \\ + [\mathrm{HBr}_2]\,\mathbf{E}(\mathrm{HBr} \to \mathrm{HBr},\, h^{*}|b^{*})\end{aligned}$$

and the interactions on pattern $h \parallel b \parallel h^{*}|b^{*}$ are

$$\exp_{\odot}(\mathcal{T}(\Pi))\mathbf{I}(h \parallel b \parallel h^{*}|b^{*}) = [\mathrm{H}_2][\mathrm{Br}_2][\mathrm{HBr}]\,\mathbf{I}\Big(\mathrm{H}_2|\mathrm{Br}_2|\mathrm{HBr} \to (\ell, m)\Big(\mathrm{H}^{(\ell)}|\mathrm{H}^{(m)}|\mathrm{Br}^{(\ell)}|\mathrm{Br}^{(m)}|\mathrm{HBr}\Big)\Big)\,.$$

## 2.3 Rate semantics for affinity networks

We will now define the rate vector $\mathcal{R}_{\mathcal{A}}([\gamma_1]\,\mathbf{I}(\gamma_1) + \ldots + [\gamma_n]\,\mathbf{I}(\gamma_n)) \in \textsc{Site}$. This gives the stoichiometric rate (that is, rate per unit reactant concentration) of the reactions at each pattern, given a vector representing the concentration of each site cluster $\gamma \in \textsc{Cluster}$ in the system.

**Definition 2.13.** The *rate vector* $\mathcal{R}_{\mathcal{A}} : \mathbb{G} \to \mathbb{S}$ for affinity network $\mathcal{A}$, is the (non-linear) function defined by

$$\mathcal{R}_{\mathcal{A}}\left(\sum_{\gamma \in \textsc{Cluster}} [\gamma]\,\mathbf{I}(\gamma)\right) = \sum_{(\gamma_1\|\ldots\|\gamma_m @ f) \in \mathcal{A}} \left(\frac{f([\gamma_1]\,, \ldots, [\gamma_m])}{[\gamma_1]\ldots[\gamma_m]}\right)\mathbf{I}(\gamma_1\| \ldots \|\gamma_m)\,.$$

This vector gives a meaningful semantics for affinity networks, which allows the reaction rates at each pattern to be computed from the site concentrations.

**Example 2.14.** In a system of mass action reactions with affinity network,

$$\mathcal{A} = \Big\{\gamma^{(i)} = \gamma_1^{(i)} \parallel \ldots \parallel \gamma_{n_i}^{(i)} \;@\; \mathrm{MA}_{r_i} : i \in I\Big\}$$

we have reaction vector,

$$\mathcal{R}_{\mathcal{A}}\Big(\sum [\gamma]\,\mathbf{I}(\gamma)\Big) = \sum_{i \in I} \frac{\mathrm{MA}_{r_i}\Big(\gamma_1^{(i)}, \ldots, \gamma_{n_i}^{(i)}\Big)}{\Big[\gamma_1^{(i)}\Big]\cdots\Big[\gamma_{n_i}^{(i)}\Big]}\mathbf{I}\Big(\gamma^{(i)}\Big) = \sum_{i \in I} r_i \mathbf{I}\Big(\gamma^{(i)}\Big)\,.$$

That is, the reaction rate vector is the vector of stoichiometric rate constants for each reaction.

**Example 2.15.** In the HBr formation process, we had affinity network,

$$\mathcal{A} = \{h \parallel b \parallel h^*|b^* \ @\ L_k\} \qquad \text{where } L_k(x_1, x_2, x_3) \triangleq \frac{x_1 x_2^{1/2}}{1 + k\frac{x_3}{x_2}}$$

and so the reaction rate vector is equal to,

$$\mathcal{R}_{\mathcal{A}}\left(\sum_{\gamma \in \textsc{Cluster}} [\gamma]\,\mathbf{I}(\gamma)\right) = \frac{L_k([h]\,,[b]\,,[h^*|b^*])}{[h][b][h^*|b^*]}\mathbf{I}(h\|b\|h^*|b^*) = \frac{[b]^{1/2}}{[h^*|b^*]\,([b] + k\,[h^*|b^*])}\mathbf{I}(h\|b\|h^*|b^*)\,.$$

Since the rates of a reaction depend on the concentrations of the reaction sites involved, this function takes as an argument a vector of the total concentrations of each site pattern in the system – these concentrations record the total concentrations of all species within a mixture which can interact at a given site, and correspond roughly to the notion of the *apparent rate* of an action in a PEPA process [5, 25]. We can define each of these concentrations inductively as,

**Definition 2.16.** The *concentration of cluster* $\gamma \in \mathbb{G}$ *in mixture* $\Pi$ is the real number $[\gamma]_\Pi$ defined by

$$[\gamma]_{[A]\cdot A} \triangleq [A]\sum_F \text{card}\Big(A \xrightarrow[\top]{\gamma} F\,, \text{trans}(A)\Big) \qquad\qquad [\gamma]_{\Pi\|\Phi} \triangleq [\gamma]_\Pi + [\gamma]_\Phi\,.$$

We then define the *site concentration vector of* $\Pi$ by,

$$\mathcal{C}(\Pi) \triangleq \sum_\gamma [\gamma]_\Pi\,\mathbf{I}(\gamma)\,.$$

The site concentration vector $\mathcal{C}(\Pi)$ can be computed compositionally based on the structure of $\Pi$ since $\mathcal{C}(\Pi \parallel \Phi) = \mathcal{C}(\Pi) + \mathcal{C}(\Phi)$. However, the following proposition shows us how $\mathcal{T}(\Pi)$ already captures the site concentrations in $\Pi$.

**Proposition 2.17.** *For any site pattern* $\gamma \in \mathcal{S}$ *and process* $\Pi$ *we have that,*

$$[\gamma]_\Pi = \|\mathcal{T}(\Pi)\mathbf{I}(\gamma)\|_1$$

*where* $\|\cdot\|_1$ *is the* $\ell^1$ *norm* $\left\|\sum_j \alpha_j \mathbf{I}(A_j \to F_j)\right\|_1 = \sum_j |\alpha_j|$.

## 2.4 Compositionality of semantics

Between the transition matrix and the rate vector we have a semantics for bond-calculus models which is compositional in both the mixture and the affinity network.

**Definition 2.18.** We define the *denotation map* $[\![\cdot]\!] : \textsc{Mix} \times \textsc{Aff} \to \mathcal{L}(\mathbb{S}, \mathbb{T}) \times (\mathbb{G} \to \mathbb{R})$ by

$$[\![(\Pi, \mathcal{A})]\!] = (\mathcal{T}(\Pi), \mathcal{R}_{\mathcal{A}}).$$

for any mixture $\Pi$ and affinity network $\mathcal{A}$.

**Theorem 2.19** (Compositionality of semantics)**.** *For mixtures* $\Pi$ *and* $\Phi$ *and affinity networks* $\mathcal{A}$, $\mathcal{B}$, *we have that,*

$$[\![(\Pi, \mathcal{A}) \parallel (\Phi, \mathcal{B})]\!] = (\mathcal{T}(\Pi) + \mathcal{T}(\Phi),\ \mathcal{R}_{\mathcal{A}} + \mathcal{R}_{\mathcal{B}})\,.$$

We end this section with an example of how we can compositionally compute the semantics when a new species is be added to an existing model.

**Example 2.20.** Suppose we introduce a new reactant into the HBr formation process, a radioactive isotope of Dibromide, ${}^{77}\mathrm{Br}_2$ [1]. This will have identical chemical properties as $\mathrm{Br}_2$ and hence can be modelled using the same reaction sites, however, the two can be distinguished since ${}^{77}\mathrm{Br}$ emits gamma rays during its radioactive decay. We can model ${}^{77}\mathrm{Br}_2$ via the new species,

$$ {}^{77}\mathrm{Br}_2 \triangleq b(\ell,m).\Big({}^{77}\mathrm{Br}^{(\ell)} \mid {}^{77}\mathrm{Br}^{(m)}\Big) \qquad\qquad {}^{77}\mathrm{Br}^{(\ell)} \triangleq b^{*}@\ell.{}^{77}\mathrm{Br}^{(\ell)} $$

(for simplicity we will not consider the effects of ${}^{77}\mathrm{Br}$ decay or any new reactions emerging from new ${}^{77}\mathrm{Br}{-}\mathrm{Br}$ and ${}^{77}\mathrm{Br}{-}\mathrm{HBr}$ complexes). Then, defining the extended system as $\Phi \triangleq \Pi \parallel \big[{}^{77}\mathrm{Br}_2\big]\,\mathrm{Br}_2$, we see the overall transition matrix is,

$$ \begin{aligned} \mathcal{T}(\Phi) &= \mathcal{T}(\Pi) + \mathcal{T}\big(\big[{}^{77}\mathrm{Br}_2\big]\,{}^{77}\mathrm{Br}_2\big) \\ &= \mathcal{T}(\Pi) + \big[{}^{77}\mathrm{Br}_2\big]\mathbf{E}\Big(\mathrm{Br}_2 \to (\ell,m)\Big({}^{77}\mathrm{Br}^{(\ell)}|{}^{77}\mathrm{Br}^{(m)}\Big),\, b\Big) \end{aligned} $$

The interactions at pattern $h \parallel b \parallel h^{*}|b^{*}$ in the extended system are now,

$$ \begin{aligned} \exp_{\odot}(\mathcal{T}(\Phi))\mathbf{I}(h \parallel b \parallel h^{*}|b^{*}) = {} & [\mathrm{H}_2][\mathrm{Br}_2][\mathrm{HBr}]\,\mathbf{I}\Big(\mathrm{H}_2|\mathrm{Br}_2|\mathrm{HBr} \to (\ell,m)\Big(\mathrm{H}^{(\ell)}|\mathrm{H}^{(m)}|\mathrm{Br}^{(\ell)}\Big)\Big) \\ & + [\mathrm{H}_2][{}^{77}\mathrm{Br}_2][\mathrm{HBr}]\,\mathbf{I}\Big(\mathrm{H}_2|{}^{77}\mathrm{Br}_2|\mathrm{HBr} \to (\ell,m)\Big(\mathrm{H}^{(\ell)}|\mathrm{H}^{(m)}|{}^{77}\mathrm{Br}^{(\ell)}\Big)\Big)\,, \end{aligned} $$

and include a new cross reaction involving the populations of $\mathrm{H}_2$ and HBr in $\Pi$ and the population of ${}^{77}\mathrm{Br}$.

The reaction rate vector $\mathcal{R}_{\mathcal{A}}$ is unchanged by the addition of the new species, however, in $\mathcal{C}(\Phi)$ the concentration of site $b$ now also includes the concentration of ${}^{77}\mathrm{Br}_2$ isotope so,

$$ \mathcal{R}_{\mathcal{A}}(\mathcal{C}(\Phi)) = \frac{\big([\mathrm{Br}_2] + \big[{}^{77}\mathrm{Br}_2\big]\big)^{1/2}}{[\mathrm{HBr}]\big([\mathrm{Br}_2] + \big[{}^{77}\mathrm{Br}_2\big] + k\,[\mathrm{HBr}]\big)}\mathbf{I}(h \parallel b \parallel h^{*}|b^{*})\,. $$

# 3 Dynamics

We will now show how the semantics defined in the previous section may be used to simulate and analyse the dynamics of a system. Firstly we will see how the combination of the transition matrix $\mathcal{T}$ and the rate vector $\mathcal{T}$ directly define the dynamics of the system when interpreted as a Chemical Reaction Network. Next we will see how to compositionally derive a more compact representation of the dynamics, in the form of the difference matrix $\mathcal{D}(\Pi) \in \mathcal{L}(\mathbb{P},\mathbb{M})$ which gives the net change in concentration for each prime species at each pattern, and can be used directly to define the dynamics of the system as a vector field,

$$ \frac{\mathrm{d}\Pi}{\mathrm{d}t} \triangleq \mathcal{D}(\Pi)\mathcal{R}_{\mathcal{A}}(\mathcal{C}(\Pi)), $$

over mixtures, specifying the instantaneous evolution of the system starting at any process vector $\Pi$ (under a given affinity network $\mathcal{A}$). Finally we will see how to symbolically derive a system of coupled differential equations which capture the dynamics of the system starting from a given initial mixture $\Pi_0$.

## 3.1 Chemical reaction network extraction

In general a bond-calculus mixture may evolve to produce infinitely many different distinct prime species – such infinite systems have been studied in the stochastic $\pi$ calculus and correspond to polymerization reactions [9]. However, given a finite initial mixture $\Pi_0$, many models will only generate finitely many prime species, allowing us to interpret the model as a Chemical Reaction Network involving finitely many species. This is possible by considering the evolution of a single generic symbolic mixture of prime species

$\Pi \triangleq \alpha_1 A_1 \parallel \ldots \parallel \alpha_n A_n$ (which we assume contains all species reachable from the initial mixture $\Pi_0$; see the supplementary material or [4, Section 3.2.4]). To do this we take the product,

$$\exp_\odot(\mathcal{T}(\Pi))\mathcal{R}_\mathcal{A}(\mathcal{C}(\Pi)) = \sum_j r_j(\boldsymbol{\alpha})\mathbf{I}(A_j \to F_j)$$

which gives the rates $r_j(\boldsymbol{\alpha})$ of each transition $A_j \to F_j$ in the system (which depend on the vector of concentrations $\boldsymbol{\alpha} = (\alpha_1, \ldots, \alpha_n)$ of each species). Then we can interpret this system as a Chemical Reaction Network [11] with reactions,

$$A_{j,1} \quad + \quad \ldots \quad + \quad A_{j,p_j} \quad \xrightarrow{r_j(\boldsymbol{\alpha})} \quad B_{j,1} \quad + \quad \ldots \quad + \quad B_{j,q_j}$$

where $\text{primes}(A_j) = \wr A_{j,1}, \ldots, A_{j,p_j} \wr$ and $\text{primes}(\text{commit}(F_j)) = \wr B_{j,1}, \ldots, B_{j,q_j} \wr$. This Chemical Reaction Network can then either be used to directly extract a system of ODEs, or interpreted stochastically as a PCTMC (Population Continuous Time Markov Chain). The bond-calculus tool supports either ODE extraction and numerical simulation via SciPy [14] or stochastic simulation via StochPy [17].

## 3.2 Difference matrix and vector field

We can also define the dynamics of the model directly, as a vector field which assigns an evolution vector $\frac{\mathrm{d}\Pi}{\mathrm{d}t}$ to each mixture $\Pi$ of species which determines the instantaneous evolution of the system from the given mixture. To this end we define the difference matrix $\mathcal{D}(\Pi)$, which represents the impact of a transition on the overall system as a difference vector $\mathcal{D}(\Pi)\mathbf{I}(\boldsymbol{\gamma}) = \sum_i \alpha_i \mathbf{I}(S_i) \in \mathbb{P}$, which captures the net change in concentration in each species resulting from the transition (assuming unit stoichiometric rate).

**Definition 3.1.** The *difference matrix* $\mathcal{D}(\Pi) \in \mathcal{L}(\mathbb{P}, \mathbb{M})$ of a mixture $\Pi$ is defined by,

$$\mathcal{D}(\Pi) = \mathcal{F} \exp_\odot(\mathcal{T}(\Pi))$$

where the *finalisation map* $\mathcal{F} \in \mathcal{L}(\mathbb{T}, \mathbb{M})$ is the linear map defined by

$$\mathcal{F}\mathbf{I}(A \to F) = \langle \text{commit}(F) \rangle - \langle A \rangle \,.$$

**Example 3.2.** For the HBr formation process, we can use the transition matrix $\mathcal{T}(\Pi)$ Example 2.12 to calculate the difference vector at the pattern $h \parallel b \parallel h^*|b^*$,

$$\begin{aligned}\mathcal{D}(\Pi)\mathbf{I}(h \parallel b \parallel h^*|b^*) &= \mathcal{F}\,[\mathrm{H}_2][\mathrm{Br}_2][\mathrm{HBr}]\,\mathbf{I}\Big(\mathrm{H}_2|\mathrm{Br}_2|\mathrm{HBr} \to (\ell, m)\Big(\mathrm{H}^{(\ell)}|\mathrm{H}^{(m)}|\mathrm{Br}^{(\ell)}|\mathrm{Br}^{(m)}|\mathrm{HBr}\Big)\Big) \\ &= [\mathrm{H}_2][\mathrm{Br}_2][\mathrm{HBr}]\,(2\mathbf{I}(\mathrm{HBr}) - \mathbf{I}(\mathrm{H}_2) - \mathbf{I}(\mathrm{Br}_2))\end{aligned}$$

since,

$$\begin{aligned}\Big\langle \text{commit}\Big((\ell, m)\Big(\mathrm{H}^{(\ell)}|\mathrm{H}^{(m)}|\mathrm{Br}^{(\ell)}|\mathrm{Br}^{(m)}|\mathrm{HBr}\Big)\Big)\Big\rangle &= \Big\langle (\nu\, \ell, m)\Big(\mathrm{H}^{(\ell)}|\mathrm{H}^{(m)}|\mathrm{Br}^{(\ell)}|\mathrm{Br}^{(m)}|\mathrm{HBr}\Big)\Big\rangle \\ &= \langle \mathrm{HBr} \mid \mathrm{HBr} \mid \mathrm{HBr} \rangle \\ &= 3\mathbf{I}(\mathrm{HBr})\end{aligned}$$

and

$$\langle \mathrm{H}_2 \mid \mathrm{Br}_2 \mid \mathrm{HBr} \rangle = \mathbf{I}(\mathrm{H}_2) + \mathbf{I}(\mathrm{Br}_2) + \mathbf{I}(\mathrm{HBr})\,.$$

We are also able to exploit the compositionality of $\mathcal{T}$ and the linearity of $\mathcal{F}$ to compute $\mathcal{D}$ compositionally (in conjunction with $\exp_\odot(\mathcal{T}(\Pi))$),

**Proposition 3.3** (Compositionality of $\mathcal{D}$). *For any pair of mixtures* $\Pi$, $\Phi$ *we have that,*

$$\begin{aligned}\mathcal{D}(\Pi \parallel \Phi) &= \mathcal{T}(\Pi) \varobar \mathcal{T}(\Phi)\\ &= \mathcal{D}(\Pi) + \mathcal{D}(\Phi) + (\exp_{\odot}(\mathcal{T}(\Pi)) - \mathbf{1}) \varobar (\exp_{\odot}(\mathcal{T}(\Phi)) - \mathbf{1})\end{aligned}$$

*where the* reaction tensor $\varobar : \mathcal{L}(\mathbb{S}, \mathbb{T}) \times \mathcal{L}(\mathbb{S}, \mathbb{T}) \to \mathcal{L}(\mathbb{S}, \mathbb{M})$ *is the bilinear map defined by,*

$$\mathbf{E}(A \to F,\, \gamma) \varobar \mathbf{E}(B \to G,\, \delta) \triangleq \mathbf{E}(\mathrm{commit}(F|G),\, \gamma\|\delta) - \mathbf{E}(A,\, \gamma\|\delta) - \mathbf{E}(B,\, \gamma\|\delta)$$

*Remark* 3.4. Similarly to the case for $\mathcal{T}(\Pi)$, an efficient implementation of the semantics may avoid computing coefficients of $\mathcal{D}(\Pi)$ which do not occur in the affinity network $\mathcal{A}$ by setting $\mathbf{E}(A \to F,\, \boldsymbol{\gamma}) \varobar \mathbf{E}(B \to G,\, \boldsymbol{\delta}) = \mathbf{0}$ whenever $\boldsymbol{\gamma} \parallel \boldsymbol{\delta} \mathbin{@} f \notin \mathcal{A}$ for some $f$.

**Example 3.5.** In the extended HBr example, we can compute the reaction matrix based on the reaction and transition matrices of the original system,

$$\begin{aligned}\mathcal{D}\big(\Pi \parallel [{}^{77}\mathrm{Br}_2]\, {}^{77}\mathrm{Br}_2\big) &= \mathcal{D}(\Pi) + \mathcal{D}\big([{}^{77}\mathrm{Br}_2]\, {}^{77}\mathrm{Br}_2\big) + \mathcal{T}(\Pi) \varobar \mathcal{T}\big([{}^{77}\mathrm{Br}_2]\, {}^{77}\mathrm{Br}_2\big)\\ &= [\mathrm{H}_2][\mathrm{HBr}]\Big([\mathrm{Br}_2](2\mathbf{E}(\mathrm{HBr},\, h\|b\|h^*|b^*) - \mathbf{E}(\mathrm{H}_2,\, h\|b\|h^*|b^*) - \mathbf{E}(\mathrm{Br}_2,\, h\|b\|h^*|b^*))\\ &\qquad + [{}^{77}\mathrm{Br}_2]\big(2\mathbf{E}\big({}^{77}\mathrm{HBr},\, h\|b\|h^*|b^*\big) - \mathbf{E}(\mathrm{H}_2,\, h\|b\|h^*|b^*) - \mathbf{E}\big({}^{77}\mathrm{Br}_2,\, h\|b\|h^*|b^*\big)\big)\Big),\end{aligned}$$

where

$$\mathrm{H}^{77}\mathrm{Br} = (\nu\, \ell)\Big(\mathrm{H}^{(\ell)} \mid {}^{77}\mathrm{Br}^{(\ell)}\Big)$$

is a newly created dynamic complex.

Finally, we may define the vector field representing the dynamics of the system.

**Definition 3.6.** The *dynamics of a model* $(\Pi, \mathcal{A})$ are defined as the vector field,

$$\frac{\mathrm{d}\Pi}{\mathrm{d}t} \triangleq \mathcal{D}(\Pi)\mathcal{R}_{\mathcal{A}}(\mathcal{C}(\Pi)).$$

This has a similar form to the dynamical equation of a Chemical Reaction Network [2, Equation 7] or to the ODE extraction equation for Bio-PEPA [10, Section 8.3], however, a key difference is that the rate laws $\mathcal{R}_{\mathcal{A}}$ are given as stoichiometric rates and depend on cluster (i.e. reaction site) concentrations rather than species concentrations whilst the matrix $\mathcal{D}(\Pi)$ contains not only the stoichiometric constants but the concentrations of each party involved in a reaction. This is what allows $\mathcal{D}$ to be computed compositionally using the multilinear functions $\odot$ and $\varobar$ (since now all of the essential nonlinearity of the system is contained in $\mathcal{R}_{\mathcal{A}}$) and is what makes it possible for a single role in a reaction (at a given cluster) to be shared between multiple species as in Example 3.8 (this corresponds to the so called *Stirling amendment* to the PEPA fluid approximation [5]).

**Example 3.7.** In the HBr formation process we have,

$$\begin{aligned}\frac{\mathrm{d}\Pi}{\mathrm{d}t} = \mathcal{D}(\Pi)\mathcal{R}_{\mathcal{A}}(\mathcal{C}(\Pi)) &= \frac{[h]_\Pi\, [b]_\Pi^{1/2}}{1 + k\frac{[h^*|b^*]_\Pi}{[b]_\Pi}}\, [\mathrm{HBr}][\mathrm{H}_2][\mathrm{Br}_2]\,(2\mathbf{I}(\mathrm{HBr}) - \mathbf{I}(\mathrm{H}_2) - \mathbf{I}(\mathrm{Br}_2))\\ &= \frac{[\mathrm{H}_2]\, [\mathrm{Br}_2]^{1/2}}{1 + k\frac{[\mathrm{HBr}]}{[\mathrm{Br}_2]}}\,(2\mathbf{I}(\mathrm{HBr}) - \mathbf{I}(\mathrm{H}_2) - \mathbf{I}(\mathrm{Br}_2))\,.\end{aligned}$$

**Example 3.8.** When we extend the system with the radioactive isotope $^{77}\mathrm{Br}_2$ as in Example 2.20, we get the overall evolution vector,

$$\begin{aligned}
\frac{\mathrm{d}\Phi}{\mathrm{d}t} &= \mathcal{D}(\Phi)\mathcal{R}_{\mathcal{A}}(\mathcal{C}(\Phi)) \\
&= \frac{\left([\mathrm{Br}_2] + \left[^{77}\mathrm{Br}_2\right]\right)_{\Pi}^{1/2}}{[\mathrm{HBr}]\left([\mathrm{Br}_2] + \left[^{77}\mathrm{Br}_2\right] + k\,[\mathrm{HBr}]\right)}[\mathrm{H}_2][\mathrm{HBr}]\Bigg([\mathrm{Br}_2](2\mathbf{I}(\mathrm{HBr}) - \mathbf{I}(\mathrm{H}_2) - \mathbf{I}(\mathrm{Br}_2)) \\
&\qquad + \left[^{77}\mathrm{Br}_2\right]\left(2\mathbf{I}\left(\mathrm{H}^{77}\mathrm{Br}\right) - \mathbf{I}(\mathrm{H}_2) - \mathbf{I}\left(^{77}\mathrm{Br}_2\right)\right)\Bigg) \\
&= \frac{[\mathrm{H}_2]\left([\mathrm{Br}_2] + \left[^{77}\mathrm{Br}_2\right]\right)^{1/2}}{1 + k\frac{[\mathrm{HBr}]}{[\mathrm{Br}_2]+\left[^{77}\mathrm{Br}_2\right]}}\Bigg(\frac{[\mathrm{Br}_2]}{[\mathrm{Br}_2] + \left[^{77}\mathrm{Br}_2\right]}(2\mathbf{I}(\mathrm{HBr}) - \mathbf{I}(\mathrm{H}_2) - \mathbf{I}(\mathrm{Br}_2)) \\
&\qquad + \frac{\left[^{77}\mathrm{Br}_2\right]}{[\mathrm{Br}_2] + \left[^{77}\mathrm{Br}_2\right]}\left(2\mathbf{I}\left(\mathrm{H}^{77}\mathrm{Br}\right) - \mathbf{I}(\mathrm{H}_2) - \mathbf{I}\left(^{77}\mathrm{Br}_2\right)\right)\Bigg).
\end{aligned}$$

This shows how the coefficients of the difference matrix and the reaction rates combine to give the rate for each individual transition: the rate of the reaction depends on the overall concentration of each site regardless of the species carrying it, whereas each of the species with a given site's involvement in the reaction is determined by what proportion of the total site concentration it comprises. This is in contrast to the mass action case considered by continuous $\pi$ where we can calculate the reaction rate for each species with a given site separately (based on the species concentration) and add up the effects due to the multilinearity of the rate law [16].

## 3.3 Symbolic ODE extraction

We have now characterized the dynamics of a system as a vector field, specifying the evolution vector $\frac{\mathrm{d}\Pi}{\mathrm{d}t}$ given any vector $\Pi \triangleq \alpha_1 A_1 \parallel \ldots \parallel \alpha_n A_n$ of species concentrations. This description involves an uncountable infinity of evolution vectors (one for each combination of species concentrations), which, whilst no problem on a theoretical level, is somewhat daunting from an implementation perspective. One way to alleviate this is abstracting $\Pi$ to a symbolic mixture $\widehat{\Pi} \triangleq [A_1]\,A_1 \parallel \ldots \parallel [A_n]\,A_n$, with variables $[A_1], \ldots, [A_n]$ for the concentration of each prime species, and calculate a symbolic evolution vector $\frac{\mathrm{d}\widehat{\Pi}}{\mathrm{d}t}$ covering the whole vector field. However, in order to capture the evolution of the system over time, the general symbolic mixture $\widehat{\Pi}$ must include all species reachable from the initial mixture $\Pi$; if species are contained in a finite dimensional subspace of $\mathbb{M}$, we can describe the dynamics of a model as a system of (finitely many) coupled differential equations. To extract this system of differential equations we first define the set of species supporting a given initial mixture.

**Definition 3.9.** For a mixture $\Pi = \sum [A]\,A \in \mathbb{M}$, the *support of* $\Pi$ is the set of prime species defined by

$$\operatorname{supp}\Pi \triangleq \Big\{A : [A] \neq 0\Big\}.$$

We now use this to define the prime species reachable from a set of species $\mathcal{S}$.

**Definition 3.10.** Given a set of prime species $\mathcal{S} \subseteq \textsc{Prime}$, we define the set of prime species reachable from $\mathcal{S}$ in $n$ steps inductively as

$$\mathrm{reach}_0(\mathcal{S}) \triangleq \mathcal{S} \qquad\qquad \mathrm{reach}_{n+1}(\mathcal{S}) \triangleq \mathrm{reach}_n(\mathcal{S}) \cup \bigcup_{\Phi \in \mathrm{span}(\mathrm{reach}_n(\mathcal{S}))} \mathrm{supp}\left(\frac{\mathrm{d}\Phi}{\mathrm{d}t}\right)$$

The *set of prime species reachable from* $\mathcal{S}$ may then be defined as,

$$\mathrm{reach}(\mathcal{S}) \triangleq \bigcup_{n=0}^{\infty} \mathrm{reach}_n(\mathcal{S}).$$

We are now ready to define the system of ODEs (with initial conditions) corresponding to a bond-calculus model.

**Definition 3.11.** Given a model $(\Pi, \mathcal{A})$ with $\Pi \triangleq \alpha_1 A_1 \parallel \ldots \parallel \alpha_n A_n$ given constant initial conditions $\alpha_1, \ldots, \alpha_n \in \mathbb{R}_{\geq 0}$, with finite set of reachable species $\text{reach}(\langle\Pi\rangle) = \{\mathbf{I}(A_1), \ldots, \mathbf{I}(A_n), \mathbf{I}(B_1), \ldots, \mathbf{I}(B_m)\}$, we abstract $\Pi$ to the symbolic mixture,

$$\widehat{\Pi} \triangleq [A_1]\, A_1 \parallel \ldots \parallel [A_n]\, A_n \parallel [B_1]\, B_1 \parallel \ldots \parallel [B_m]\, B_m.$$

Then we define the system of ODEs (with initial conditions) corresponding to $(\Pi, \mathcal{A})$ as,

$$\begin{aligned} \frac{\mathrm{d}[A_i]}{\mathrm{d}t} &= f_i([A_1], \ldots, [A_n], [B_1], \ldots, [B_m]) \qquad & [A_i]_0 &= \alpha_i \qquad & (i = 1, \ldots, n) \\ \frac{\mathrm{d}[B_j]}{\mathrm{d}t} &= g_j([A_1], \ldots, [A_n], [B_1], \ldots, [B_m]) \qquad & [B_j]_0 &= 0 \qquad & (j = 1, \ldots, m) \end{aligned}$$

where

$$\frac{\mathrm{d}\widehat{\Pi}}{\mathrm{d}t} = \sum_{i=1}^{n} f_i([A_1], \ldots, [A_n], [B_1], \ldots, [B_m])\mathbf{I}(A_i) + \sum_{j=1}^{m} g_j([A_1], \ldots, [A_n], [B_1], \ldots, [B_m])\mathbf{I}(B_j)\,.$$

In fact, our compositonal semantics gives Algorithm 1, an efficient procedure for deriving the extended symbolic process $\widehat{\Pi}$ and its evolution vector.

**Example 3.12.** In the HBr system we have $\text{reach}(\text{supp}(\Pi)) = \text{supp}(\Pi) = \{\mathbf{I}(\mathrm{H}_2), \mathbf{I}(\mathrm{Br}_2), \mathbf{I}(\mathrm{HBr})\}$ and so this model corresponds to a system of three ODEs,

$$\frac{\mathrm{d}[\mathrm{H}_2]}{\mathrm{d}t} = \frac{\mathrm{d}[\mathrm{Br}_2]}{\mathrm{d}t} = -\frac{[\mathrm{H}_2]\,[\mathrm{Br}_2]^{1/2}}{1 + k\frac{[\mathrm{HBr}]}{[\mathrm{Br}_2]}} \qquad \frac{\mathrm{d}[\mathrm{HBr}]}{\mathrm{d}t} = \frac{2\,[\mathrm{H}_2]\,[\mathrm{Br}_2]^{1/2}}{1 + k\frac{[\mathrm{HBr}]}{[\mathrm{Br}_2]}}.$$

**Example 3.13.** Whilst previously we included the dynamic complex $\mathrm{HBr} \triangleq (\nu\, \ell)\Big(\mathrm{H}^{(\ell)} \mid \mathrm{B}^{(\ell)}\Big)$ explicitly in the definition of the Hydrogen Dibromide formation process, this was not in fact necessary. Suppose instead we had,

$$\Phi \triangleq [\mathrm{H}_2]_0\, \mathrm{H}_2 \parallel [\mathrm{Br}_2]_0\, \mathrm{Br}_2$$

**Input:** Initial symbolic mixture $\widehat{\Pi} \triangleq [A_1]\, A_1 \parallel \ldots \parallel [A_n]\, A_n$ and affinity network $\mathcal{A}$.
**Output:** A pair $\left(\widehat{\Pi}, \frac{\mathrm{d}\widehat{\Pi}}{\mathrm{d}t}\right)$ of a symbolic mixture $\widehat{\Pi}$ and its evolution vector $\frac{\mathrm{d}\widehat{\Pi}}{\mathrm{d}t}$.
**while** $\text{supp}\Big(\frac{\mathrm{d}\widehat{\Pi}}{\mathrm{d}t}\Big) \not\subseteq \text{supp}\big(\widehat{\Pi}\big)$ **do**

  Pick some $B \in \text{supp}\left(\frac{\mathrm{d}\widehat{\Pi}}{\mathrm{d}t}\right) \setminus \text{supp}\big(\widehat{\Pi}\big)$;
  $\widehat{\Pi}' := \widehat{\Pi} \parallel [B]\, B$;
  $\exp_{\odot}(\mathcal{T}(\widehat{\Pi}')) := \exp_{\odot}(\mathcal{T}(\widehat{\Pi})) \odot \exp_{\odot}(\mathcal{T}([B]\, B))$;
  $\mathcal{D}(\widehat{\Pi}') := \mathcal{D}(\widehat{\Pi}) + \mathcal{D}([B]\, B) + (\exp_{\odot}(\mathcal{T}(\widehat{\Pi})) - \mathbf{1}) \varobar (\exp_{\odot}(\mathcal{T}([B]\, B)) - \mathbf{1})$;
  $\mathcal{C}(\widehat{\Pi}') := \mathcal{C}(\widehat{\Pi}) + \mathcal{C}([B]\, B)$;
  $\frac{\mathrm{d}\widehat{\Pi}'}{\mathrm{d}t} := \mathcal{D}(\widehat{\Pi}')\mathcal{R}_{\mathcal{A}}(\mathcal{C}(\widehat{\Pi}'))$;

**end**

**Algorithm 1:** Mixture expansion algorithm. We utilize Propositions 3.3 and 2.9 to compute only the new terms of $\mathcal{D}$ at each step.

then HBr appears dynamically in $\frac{\mathrm{d}\Phi}{\mathrm{d}t}$ giving

$$\begin{aligned}
\mathrm{reach}_0(\mathrm{supp}(\Phi)) &= \mathrm{span}\{\mathbf{I}(\mathrm{H}_2)\,, \mathbf{I}(\mathrm{Br}_2)\} \\
\mathrm{reach}_1(\mathrm{supp}(\Phi)) &= \mathrm{span}\{\mathbf{I}(\mathrm{H}_2)\,, \mathbf{I}(\mathrm{Br}_2)\,, \mathbf{I}(\mathrm{HBr})\} \\
\mathrm{reach}_2(\mathrm{supp}(\Phi)) &= \mathrm{span}\{\mathbf{I}(\mathrm{H}_2)\,, \mathbf{I}(\mathrm{Br}_2)\,, \mathbf{I}(\mathrm{HBr})\} \\
\vdots \qquad &= \qquad \vdots
\end{aligned}$$

and hence

$$\mathrm{reach}(\mathrm{supp}(\Phi)) = \mathrm{span}\{\mathbf{I}(\mathrm{H}_2)\,, \mathbf{I}(\mathrm{Br}_2)\,, \mathbf{I}(\mathrm{HBr})\}.$$

Therefore $\widehat{\Phi} = \widehat{\Pi}$ and we get the same ODEs as in the previous example with initial condition $[\mathrm{HBr}]_0 = 0$.

# References


[1] National Center for Biotechnology Information. PubChem Compound Database; CID=177674, `https://pubchem.ncbi.nlm.nih.gov/compound/177674` (accessed Jan. 8, 2018).

[2] David Angeli. A tutorial on chemical reaction network dynamics. *European journal of control*, 15(3-4):398–406, 2009.

[3] Ron Ausbrooks, Stephen Buswell, David Carlisle, Giorgi Chavchanidze, Stéphane Dalmas, Stan Devitt, Angel Diaz, Sam Dooley, Roger Hunter, Patrick Ion, et al. Mathematical markup language (mathml) version 3.0. Technical report, Tech. rep. World Wide Web Consortium (W3C), 2010. url: `http://www.w3.org/TR/MathML3`, 2010.

[4] Chris Banks. *Spatio-temporal Logic for the Analysis of Biochemical Models.* PhD thesis, Edinburgh, 2016. Supervised by Ian Stark.

[5] Soufiene Benkirane, Jane Hillston, Chris McCaig, Rachel Norman, and Carron Shankland. Improved continuous approximation of pepa models through epidemiological examples. *Electronic Notes in Theoretical Computer Science*, 229(1):59–74, 2009.

[6] Max Bodenstein and SC Lind. Geschwindigkeit der bildung des bromwasserstoffs aus seinen elementen. *Zeitschrift für Physikalische Chemie*, 57(1):168–192, 1907.

[7] Nadia Busi, Maurizio Gabbrielli, and Gianluigi Zavattaro. Replication vs. recursive definitions in channel based calculi. In *Automata, Languages and Programming: 30th International Colloquium, ICALP 2003, Eindhoven, The Netherlands, June 30-July 4, 2003. Proceedings*, volume 2719, page 133. Springer, 2003.

[8] Luca Cardelli. On process rate semantics. *Theoretical Computer Science*, 391(3):190 – 215, 2008. Converging Sciences: Informatics and Biology.

[9] Luca Cardelli, Emmanuelle Caron, Philippa Gardner, Ozan KahramanoÄ§ullarÄś, and Andrew Phillips. A process model of actin polymerisation. *Electronic Notes in Theoretical Computer Science*, 229(1):127 – 144, 2009. Proceedings of the Second Workshop From Biology to Concurrency and Back (FBTC 2008).

[10] Federica Ciocchetta and Jane Hillston. Bio-PEPA: A framework for the modelling and analysis of biological systems. *Theoretical Computer Science*, 410(33):3065 – 3084, 2009.

[11] Jeremy Gunawardena. Chemical reaction network theory for in-silico biologists. 2003.

[12] Jane Hillston. Fluid flow approximation of pepa models. In *Quantitative Evaluation of Systems, 2005. Second International Conference on the*, pages 33–42. IEEE, 2005.

[13] Jane Hillston and Leïla Kloul. An efficient kronecker representation for pepa models. In *Process Algebra and Probabilistic Methods. Performance Modelling and Verification*, pages 120–135. Springer, 2001.

[14] Eric Jones, Travis Oliphant, Pearu Peterson, et al. SciPy: Open source scientific tools for Python, 2001–. [Online; accessed 12-02-2018].

[15] Marek Kwiatkowski. *A formal computational framework for the study of molecular evolution.* PhD thesis, Edinburgh, 2010. Supervised by Ian Stark.

[16] Marek Kwiatkowski and Ian Stark. The continuous $\pi$-calculus: A process algebra for biochemical modelling. In *Computational Methods in Systems Biology: Process of the Sixth International Conference CMSB 2008*, number 5307 in Lecture Notes in Computer Science, pages 103–122. Springer-Verlag, 2008.

[17] Timo R. Maarleveld, Brett G. Olivier, and Frank J. Bruggeman. StochPy: A comprehensive, user-friendly tool for simulating stochastic biological processes. *PLOS ONE*, 8(11):1–10, 11 2013.

[18] Robin Milner. The polyadic $\pi$-calculus: a tutorial. In *Logic and algebra of specification*, pages 203–246. Springer, 1993.

[19] Robin Milner. *Communicating and mobile systems: the $\pi$-calculus.* Cambridge university press, 1999.

[20] Catuscia Palamidessi and Frank Valencia. Recursion vs replication in process calculi: Expressiveness. *Bulletin-European Association for Theoretical Computer Science*, 87:105–125, 2005.

[21] Gordon D Plotkin. A structural approach to operational semantics. 1981.

[22] C. Priami. Stochastic $\pi$-calculus. *The Computer Journal*, 38(7):578–589, 1995.

[23] Michael Rettelbach and Markus Siegle. Compositional minimal semantics for the stochastic process algebra tipp. In *Proc. of 2nd Process Algebra and Performance Modelling Workshop*, page 143, 1994.

[24] Davide Sangiorgi. $\pi$-calculus, internal mobility, and agent-passing calculi. *Theoretical Computer Science*, 167(1-2):235–274, 1996.

[25] Mirco Tribastone, Stephen Gilmore, and Jane Hillston. Scalable differential analysis of process algebra models. *IEEE Transactions on Software Engineering*, 38(1):205–219, 2012.
